# Supplementary material for: Testing Credibility of Public and Private Surveys through the Lens of Regression
Source: arXiv:2410.05458 source file (2024-10-07)
Supplement: Supplementary file 1 [file 1_LDP_Proofs.tex]

\subsubsection{\dppair-Local Differential Privacy}
\begin{lemma}[Learning from data with additive subgaussian noise~\cite{LDP_Regression_AOS}]\label{lemma: Additive Subgaussian noise regression}
    Given a linear regression problem of the form $\response = \inn{\coeff}{\covariate} + \regnoise, \covariate \in \R^d$ with optimal solution $\coeff^*$ where we observe $\noisycovariate = \covariate + \noisevariable$ and $\covariate,\noisevariable$ are $\sigma_\covariate^2,\sigma_\noisevariable^2$ (resp.) subgaussian random vectors, the algorithm \ref{Algorithm: LDP Survey Regression} learns $\coeffhat$ using $n \geq \frac{(\sigma_\covariate^2+\sigma_\regnoise^2)^2}{\lambda^2_{min}(\xvariance)}d\log{d}$ samples such that for some constants $\constant_1,\constant_2$, with probability at least $1 - d^{-\constant_1}$, we have:
    \[\norm{\coeffhat-\coeff^*}_2 \leq \constant_2 \frac{\sigma_\noisycovariate(\sigma_\noisevariable+\sigma_\epsilon)}{\lambda_{min}(\xvariance)}\norm{\coeff^*}_2\sqrt{\frac{d\log{d}}{n}}\]
\end{lemma}

We use the Lemma \ref{lemma: Gaussian LDP Survey} and \ref{lemma: Additive Subgaussian noise regression} to prove the Theorem \ref{Theorem: Learning from Gaussian LDP data}:

\begin{proof}[Proof of Theorem \ref{Theorem: Learning from Gaussian LDP data}]
    Under the conditions stated in the theorem, \ref{lemma: Gaussian LDP Survey} ensures that $\AlgoPriv$ outputs $\surveyset'$ satisfying \dppair-privacy and the variance of noise $\Sigma_\noisevariable = \frac{\constant_1\boundonx\sqrt{\log\frac{1}{\dpdelta}}}{\dpepsilon}\identity$. This ensures that the noise $\noisevariable$ is a $\frac{\constant_1\boundonx\sqrt{\log\frac{1}{\dpdelta}}}{\dpepsilon}$-subgaussian random vector. The random vector $\covariate$ is bounded as $|\covariate_i|\leq \boundonx$, and hence $2\boundonx$-subgaussian. This gives us the upper bound on $\norm{\coeff^*-\coeffhat}_2$ as:
    
    \[\constant_2\frac{\boundonx\sqrt{\frac{\log\left(\frac{1}{\dpdelta}\right)}{\dpepsilon}+1}\left(\frac{\boundonx\sqrt{\log\left(\frac{1}{\dpdelta}\right)}}{\dpepsilon}+\sigma_\regnoise\right)}{\lambda_{min}(\xvariance)}\norm{\coeff^*}_2\sqrt{\frac{d\log{d}}{n}}\]
    
    Putting in the upper bound on $\norm{\coeff^*}_2$ as $\linweight$ gives the bound.
\end{proof}

% -----------------------------------New Subsection-----------------------------------

\subsubsection{$\dpepsilon$-Local Differential Privacy}

\begin{theorem}\label{Theorem: Larger Deviation Noisy Regression}
    Given a linear regression problem of the form $\response = \inn{\coeff}{\covariate} + \regnoise, \covariate \in \R^d$ with optimal solution $\coeff^*$ where we observe $\noisycovariate = \covariate + \noisevariable$, algorithm \ref{Algorithm: LDP Survey Regression} or its corresponding Lagrangian version satisfies the following bounds if there exists  $\Phi(\noisycovariatematrix)$ such that $\norm{\predcovardummy - \basecovardummy\coeff^*}_\infty \leq \Phi(\noisycovariatematrix)\frac{\log^2d}{n}$, and the matrix $\basecovardummy$ satisfies for all $\coeff \in \R^d$, $\coeff^T\basecovardummy\coeff \geq \lowerrealpha \norm{\coeff}_2^2-\tau(n,d)\norm{\coeff}_1^2$ for some $\lowerrealpha > 0$ and $\tau(n,d) > 0$ with $\tau(n,d) \leq \frac{\lowerrealpha}{2d}$:
    \begin{align}
        \norm{\coeffhat-\coeff^*}_2 \leq \frac{\constant\sqrt{d}}{\lowerrealpha}\Phi(\noisycovariatematrix)\frac{\log^2d}{n}
    \end{align}
    Where $\constant$ is a constant. The $\lagrangian_n$ for the Lagrangian version must be fixed such that $\lagrangian_n \geq \Phi(\noisycovariatematrix)\frac{\log^2d}{n}$.

    \begin{proof}
        Let us consider the loss function 
        \begin{align*}
        \sL(\coeff) = \frac{1}{2}\coeff^T\basecovardummy\coeff - \inn{\predcovardummy}{\coeff}+\lagrangian_n\norm{\coeff}_1
        \end{align*}
        Note that this recovers both the constrained and lagrangian formulation by fixing $\lagrangian_n$ appropriately. We obtain our solution correspondingly as:
        \[\widehat{\coeff} = \argmin \frac{1}{2}\coeff^T\basecovardummy\coeff - \inn{\predcovardummy}{\coeff}+\lagrangian_n\norm{\coeff}_1\]
        Let $\coeff^*$ be the solution to the regression vector. And denote by $\nuvector := \widehat{\coeff} - \coeff^*$. Due to optimality of $\coeffhat$, we have $\sL(\coeffhat) \leq \sL(\coeff^*)$, which can be reformulated as:
        \begin{align}
        \frac{1}{2}\nuvector^t\basecovardummy\nuvector &\leq \inn{\nuvector}{\predcovardummy - \basecovardummy\coeff^*}+\lagrangian_n\left(\norm{\coeff^*}_1 - \norm{\coeff^*+\nuvector}\right)\label{Base Ineq Thm: Laplace LDP Stat}    
        \end{align}
We start with providing an upper bound on the Inequality \ref{Base Ineq Thm: Laplace LDP Stat}. By our assumption on $\norm{\predcovardummy - \basecovardummy\coeff^*}_\infty$, we have for the first term:
        \begin{align*}
            \inn{\nuvector}{\predcovardummy - \basecovardummy\coeff^*}     
                            &\leq \norm{\nuvector}_1\norm{\predcovardummy - \basecovardummy\coeff^*}_\infty\\
                            &\leq \norm{\nuvector}_1\Phi(\noisycovariatematrix)\frac{\log^2d}{n}\\
                            &\leq \sqrt{d}\norm{\nuvector}_2\Phi(\noisycovariatematrix)\frac{\log^2d}{n}
        \end{align*}
        Where the first inequality follows from Holder's inequality. For the second term, we have:
        \begin{align*}
            \lagrangian_{n}(\norm{\coeff^*}_{1} - \norm{\coeff^*+\nuvector}_1)
            \leq \lagrangian_{n}  \norm{\nuvector}_{1}
            \leq \lagrangian_{n} \sqrt{d} \norm{\nuvector}_{2}
        \end{align*}
        Here, the first inequality follows from Triangle Inequality. Hence, by our choice of $\lagrangian_n$, the right hand side of inequality \ref{Base Ineq Thm: Laplace LDP Stat} can be upper bounded by:
        \begin{align}
            2\sqrt{d}\Phi(\noisycovariatematrix)\frac{\log^2d}{n}\norm{\nuvector}_2\label{Ineq: Base Right hand upperbound Thm: Laplace LDP Stat}
        \end{align}
        Now we focus on lower bounding the left hand side of the inequality:
        \begin{align}
           \nonumber \nuvector^T\basecovardummy\nuvector \geq& \lowerrealpha\norm{\nuvector}_2^2- \tau(n,d)\norm{\nuvector}_1^2\\
           \nonumber \geq& \left(\lowerrealpha - d\tau(n,d)\right)\norm{\nuvector}_2^2\\
            \geq& \frac{\lowerrealpha}{2}\norm{\nuvector}_2^2 \label{Ineq: Base Left hand lowerbound Thm: Laplace LDP Stat}
        \end{align}
        Where the first inequality follows from the lower restricted eigenvalue condition on $\basecovardummy$ and the second inequality follows from the assumption $\lowerrealpha \geq 2d\tau(n,d)$. Combining the inequalities \ref{Base Ineq Thm: Laplace LDP Stat}, \ref{Ineq: Base Left hand lowerbound Thm: Laplace LDP Stat} and \ref{Ineq: Base Right hand upperbound Thm: Laplace LDP Stat}, we obtain:
        \begin{align*}
            \frac{\lowerrealpha}{2}\norm{\nuvector}_{2}^2 \leq 2\sqrt{d}\Phi(\noisycovariatematrix)\frac{\log^2d}{n}\norm{\nuvector}_2
            \norm{\nuvector}_2 \leq \frac{\constant_0\sqrt{d}}{\lowerrealpha}\Phi(\noisycovariatematrix)\frac{\log^2d}{n}
        \end{align*}
    \end{proof}
\end{theorem}

Observe that the Theorem \ref{Theorem: Larger Deviation Noisy Regression} is a deterministic result. We would like to show that the conditions stated in the theorem hold with high probability in certain problem settings. We formalize this idea in the following theorem:

To prove the stated theorem, we use the following results from \cite{LDP_Regression_AOS}:

\begin{lemma}\label{lemma: RE conditions reduction}
    Suppose $s \geq 1$ and $\basecovardummy$ is an estimator of $\Sigma_x$ satisfying the deviation conditions:
    \[|\coeff^T(\basecovardummy-\xvariance)\coeff| \leq \frac{\lambda_{min}(\xvariance)}{54} \hfill \forall \coeff \in \bK(2s)\]
    Then we have the lower-RE condition:
    \[\coeff^T\basecovardummy\coeff \geq \frac{\lambda_{min}(\xvariance)}{2}\norm{\coeff}_2^2-\frac{\lambda_{min}(\xvariance)}{2s}\norm{\coeff}_1^2\]
    Where $\lambda_{min}(\mathbf{M})$ denotes the least eigenvalues of the matrix $M$. And $\bK(2s):= \bfB_0(s)\cap \bfB_2(1)$ where $\bfB_p(r)$ denote balls of radius $r$ in $p$-dimensional box.
\end{lemma}

\begin{lemma}\label{lemma: ball bound laplace}
    If $\covariatematrix \in \R^{n\times d}$ is a random matrix whose each entry are i.i.d. such that $\Pr(x_i \geq t) \leq \exp\left(-\frac{t}{\constant_x}\right)$, then there is a universal constant $\constant$ such that:
    \begin{align*}
    &\Pr\left[\sup_{\coeff \in \bK(2s)}\left|\frac{\norm{\covariatematrix\coeff}_2^2}{n}-\E\left[\frac{\norm{\covariatematrix\coeff}_2^2}{n}\right]\right|\geq t\right] \\&\leq \constant\exp\left(-\frac{\sqrt{nt}}{\constant_\covariate}+2s\log d\right)
    \end{align*}
\end{lemma}

Now, we use these results to show that the assumptions stated in Theorem \ref{Theorem: Larger Deviation Noisy Regression} hold with high probability under the conditions stated in \ref{Theorem: Sub-Expoential Noise Noisy Regression}:

% \begin{theorem}\label{Theorem: Sub-Expoential Noise Noisy Regression}
%     Given a linear regression problem of the form $\response = \inn{\coeff}{\covariate} + \regnoise, \covariate \in \R^d$ with optimal solution $\coeff^*$ where we observe $\noisycovariate = \covariate + \noisevariable$ and $\covariate$ comes from a distribution such that $\Pr(X_i \geq t) \leq \exp\left(-\frac{t}{\constant_\covariate}\right)$, $\regnoise$ comes from a distribution such that $\Pr(\regnoise \geq t) \leq \exp\left(-\frac{t}{\constant_\regnoise}\right)$, and $\noisevariable$ comes from a distribution such that $\Pr(\noboldnoisevariable_i \geq t) \leq \exp\left(-\frac{t}{\constant_\noisevariable}\right)$, algorithm \ref{Algorithm: LDP Survey Regression} or its corresponding Lagrangian version with $n \geq \max\left(\frac{\constant_\noisycovariate}{\lambda_{min}(\xvariance)},1\right)d^2\log^2d$ satisfies:
%     \[
%     \norm{\coeffhat-\coeff^*}_2 \leq \frac{\constant_1\sqrt{d}}{\lambda_{min}(\xvariance)}\constant_{max}\norm{\coeff^*}_2\frac{\log^2d}{n}
%     \]
%     With probability at least $1 - \frac{1}{d^{\constant_2}}$ for some constants $\constant_1$ and $\constant_2$, where $\constant_z = \constant_\covariate+\constant_\noisevariable$ and $\constant_{max} = \max(\constant_\covariate,\constant_\noisevariable,\constant_\regnoise)$.
% \end{theorem}

\begin{lemma}\label{lemma: Restricted Eigenvalue}
    Under the conditions of theorem \ref{Theorem: Sub-Expoential Noise Noisy Regression}, we have the lower-RE condition satisfied with $\lowerrealpha = \frac{\lambda_{min}(\xvariance)}{2}$ and $\tau(n,p) = c_0 \lambda_{min}(\xvariance)\max\left(\frac{\constant_\noisycovariate}{\sqrt{\lambda_{min}(\xvariance)}} , 1 \right) \frac{\log d}{\sqrt{n}}$ with probability at least $1-\constant\exp\left(-\sqrt{n}\min\left(\frac{\sqrt{\lambda_{min}(\xvariance)}}{\lambda},2\right)\right)$

    \begin{proof}
        By Lemma \ref{lemma: RE conditions reduction}, and the fact that $\basecovardummy - \xvariance = \frac{\noisycovariatematrix^T\noisycovariatematrix}{n}-\zvariance$, we can fix $s = \frac{1}{\constant_1}\frac{\sqrt{n}}{\log d}\max\left(\frac{\constant_\noisycovariate}{\sqrt{\lambda_{min}(\xvariance)}},1\right)$ to obtain the stated bound if $\sup_{\coeff\in\bK(2s)} \left|\coeff^T\left(\frac{\noisycovariatematrix^T\noisycovariatematrix}{n}-\zvariance\right)\coeff\right| \leq \frac{\lambda_{min}(\xvariance)}{54}$. Hence, it suffices to show that this bound holds with high probability. Note that $\noisycovariatematrix$ satisfies the condition of lemma \ref{lemma: ball bound laplace} with $\constant_\noisycovariate = \constant_\covariate + \constant_\noisevariable$.

        \begin{align*}
            &\Pr\left[\sup_{\coeff\in\bK(2s)} \left| 
            \coeff^T  \left(\frac{\noisycovariatematrix^T\noisycovariatematrix}{n}-\zvariance\right)\coeff\right| \geq t\right] \\
            \leq &\constant_2 \exp\left(-\frac{\sqrt{nt}}{\constant_\noisycovariate}+2s\log d\right)\\
            \leq &\constant_2\exp\left(-\sqrt{n}\min\left(\frac{\sqrt{\lambda_{min}(\xvariance)}}{\constant_\noisycovariate},1\right)\right)
        \end{align*}
        Where the first inequality follows from lemma \ref{lemma: ball bound laplace} and the second inequality follows from fixing $t = \frac{\lambda_{min}(\xvariance)}{54}$.
    \end{proof}
\end{lemma}

\begin{lemma}\label{Lemma: Bounded Deviation}
    Under the conditions of Theorem \ref{Theorem: Sub-Expoential Noise Noisy Regression}, the deviation bound condition on $\norm{\predcovardummy - \basecovardummy\coeff^*}_\infty$ is satisfied by:
    \[
    \Phi(\noisycovariatematrix) \leq \constant_1\constant_{max}\norm{\coeff^*}_2
    \]
    with probability at least $1 - \frac{1}{d^{\constant_2}}$ where $\constant_1,\constant_2$ are constants, and $\constant_{max} = \max(\constant_\covariate,\constant_\noisevariable,\constant_\regnoise)$.

    \begin{proof}
        We use the model assumption $\response = \inn{\coeff}{\covariate} + \regnoise$ to upper bound $\norm{\predcovardummy - \basecovardummy\coeff^*}_\infty$:
        \begin{align*}
            \norm{\predcovardummy - \basecovardummy\coeff^*}_\infty &= \norm{\frac{\noisycovariatematrix^T \responsevector}{n}-\left(\frac{\noisycovariatematrix^T\noisycovariatematrix}{n}-\wvariance
        \right)\coeff^*}\\
            &= \norm{\frac{\noisycovariatematrix^T(\covariatematrix\coeff^*+\regnoisevector)}{n}-\left(\frac{\noisycovariatematrix^T\noisycovariatematrix}{n}-\wvariance\right)\coeff^*}_\infty\\
            &= \norm{\frac{\noisycovariatematrix^T\regnoisevector}{n}-\left(\frac{\noisycovariatematrix^T(\noisycovariatematrix-\covariatematrix)}{n}-\wvariance\right)\coeff^*}_\infty\\
            &= \norm{\frac{\noisycovariatematrix^T\regnoisevector}{n}+\left(\wvariance-\frac{\noisycovariatematrix^T\mathbf{W}}{n}\right)\coeff^*}_\infty\\
            &\leq \norm{\frac{\noisycovariatematrix^T\regnoisevector}{n}}_\infty + \norm{\left(\wvariance-\frac{\noisycovariatematrix^T\mathbf{W}}{n}\right)\coeff^*}_\infty
        \end{align*}
        Consequently lemma \ref{Lemma: Laplace Squared Tail} completes the proof.
    \end{proof}
\end{lemma}

    \begin{proof}[Proof of Theorem \ref{Theorem: Sub-Expoential Noise Noisy Regression}]
        The lemma \ref{lemma: Restricted Eigenvalue} and \ref{Lemma: Bounded Deviation} ensures that the deviation condition and restricted eigenvalues are satisfied with $\lowerrealpha = \frac{\lambda_{min}(\xvariance)}{2}$ under the conditions given. Additionally, fixing $n \geq \max\left(\frac{\constant_\noisycovariate}{\lambda_{min}(\xvariance)},1\right)d^2\log^2d$ ensures the success probabilities are at least $1 - \frac{1}{d^{\constant_2}}$, as well as $\tau(n,d) \leq \frac{\lowerrealpha}{2d}$.
    \end{proof}

    \begin{proof}[Proof of Theorem \ref{Theorem: Learning from Laplacian LDP data}]
        Under the conditions stated in the theorem, \ref{lemma: Laplace LDP Survey} ensures that $\AlgoPriv$ outputs $\surveyset'$ satisfying $\dpepsilon$-privacy and the variance of noise $\noisevariance = \frac{8\boundonx^2}{\dpepsilon^2}$. Additionally the noise variables $\noisevariable$ satisfies the condition of Theorem \ref{Theorem: Sub-Expoential Noise Noisy Regression} with $\constant_\noisevariable = \frac{2\boundonx}{\dpepsilon}$. Also, the bounded domain assumption on $\covariate$ ensures it satisfies the conditions with $\constant_\covariate = \boundonx^2$. Putting these values in Theorem \ref{Theorem: Sub-Expoential Noise Noisy Regression}, we get that with probability $1- \frac{1}{d^{\constant_1}}$ , $\norm{\coeff^*-\coeffhat}_2$ is upper bounded by:
        \[
        \frac{\constant_2\sqrt{d}}{\lambda_{min}(\xvariance)}\max\left(\frac{\boundonx}{\dpepsilon},\boundonx, \constant_\regnoise\right)\norm{\coeff^*}_2\frac{\log^2d}{n}
        \]
    \end{proof}

\begin{proof}[Proof of Theorem \ref{Theorem: Learning from Laplacian LDP data}]
        Under the conditions stated in the theorem, \ref{lemma: Laplace LDP Survey} ensures that $\AlgoPriv$ outputs $\surveyset'$ satisfying $\dpepsilon$-privacy and the variance of noise $\noisevariance = \frac{8\boundonx^2}{\dpepsilon^2}$. Additionally the noise variables $\noisevariable$ satisfies the condition of Theorem \ref{Theorem: Sub-Expoential Noise Noisy Regression} with $\constant_\noisevariable = \frac{2\boundonx}{\dpepsilon}$. Also, the bounded domain assumption on $\covariate$ ensures it satisfies the conditions with $\constant_\covariate = \boundonx^2$. Putting these values in Theorem \ref{Theorem: Sub-Expoential Noise Noisy Regression}, we get that with probability $1- \frac{1}{d^{\constant_1}}$ , $\norm{\coeff^*-\coeffhat}_2$ is upper bounded by:
        \[
        \frac{\constant_2\sqrt{d}}{\lambda_{min}(\xvariance)}\max\left(\frac{\boundonx^2}{\dpepsilon^2},\boundonx^2, \constant_\regnoise\right)\norm{\coeff^*}_2\frac{\log^2d}{n}
        \]
\end{proof}
